# Supplementary material for: CUTS+: High-dimensional Causal Discovery from Irregular Time-series
Source: arXiv:2305.05890 ancillary file (2023-08-16)
Supplement: Supplementary file 1 [file CUTS_Plus_Supp_ver0816.pdf]

# Supplementary Material for "CUTS+: High-dimensional Causal Discovery from Irregular Time-series"

August 15, 2023

## A Theorems and Proof

In the following, we prove the convergence of the GCPG $\mathbf{Q} = \sigma(\Theta)$.

**Assumption 1** *Time-series $i$ sampled at time $t$, denoted as $x_{i,t} \in \mathbb{R}$ is generated with the Structural Causal Model (SCM), i.e., $x_{i,t} = f_i(\mathbf{x}_{1,t-\tau:t-1}, \mathbf{x}_{2,t-\tau:t-1}, ..., \mathbf{x}_{N,t-\tau:t-1}) + e_{i,t}, \quad i = 1, 2, ..., N$. Where $\tau$ denotes the maximal time lag.*

**Assumption 2** *Component $i$ of CDNN $f_{\phi_i}$ approximate generative function $f_i$ with an error smaller than $e_{NN,i}$.*

This assumption is satisfied if we leverage the Universal Approximation Theorem of Neural Networks [1]. It is reasonable since we can learn the dynamics under time-series well with our deep neural network.

**Assumption 3** $\exists \lambda_0, \forall i, j = 1, ..., N, \left| f_{\phi_j}(\mathbf{X} \odot \mathbf{s}_{:,j|\mathcal{G}_k=1}) - f_{\phi_j}(\mathbf{X} \odot \mathbf{s}_{:,j|\mathcal{G}_k=0}) \right| \leq \lambda_0$ *if and only if group $\mathbf{X}_{\mathcal{G}_k}$ Granger does not cause $\mathbf{x}_j$, where $\mathbf{s}_{:,j|j=r}$ is vector $\mathbf{s}_{:,j}$ with element $\mathbf{s}_{ij} = r, \forall i \in \mathcal{G}_k$.*

Here we define $f_{\phi_j}(\mathbf{X} \odot \mathbf{s}_{:,j}) \triangleq f_{\phi_j}(\{\mathbf{x}_1 \cdot s_{1j}, ..., \mathbf{x}_N \cdot s_{Nj}\})$ (note that this is not the standard definition of Hadamard product, because $\mathbf{X}$ is 2-dimensional). This assumption can be regarded as a relaxation of Definition 2, i.e.,

$$|f_j(\{\mathbf{X}_{\mathcal{G}_i}, \mathbf{X} \backslash \mathbf{X}_{\mathcal{G}_i}\}) - f_j(\{\mathbf{0}, \mathbf{X} \backslash \mathbf{X}_{\mathcal{G}_i}\})| \leq \lambda_0 \quad (1)$$

With these assumptions, the grouping version of Theorem 1 in [2] can be formulated as

**Theorem 1** *There exists a penalty coefficient $\lambda$, s.t. GCPG element $q_{kj}$ decrease towards 0 if group $\mathbf{X}_{\mathcal{G}_k}$ does not Granger cause time-series $j$, $q_{kj}$ increase towards 1 if group $\mathbf{X}_{\mathcal{G}_k}$ Granger cause time-series $j$.*

**Proof.** The learned CPG $\tilde{\mathbf{M}} = \mathbf{G}^T \mathbf{Q}$, and $\tilde{\mathbf{m}}_{ij} = \mathbf{g}_{:,i}^T \mathbf{q}_{:,j}$. Since each time-series is and can only be allocated to one group, we get

$$\mathbf{s}_{:,j} = \mathbf{G}^T \mathbf{s}'_{:,j}, \quad \mathbf{s}'_{:,j} \sim Ber(\sigma(\theta_{:,j})) \quad (2)$$

The loss function in ***Causal Discovery Stage*** is

$$\mathcal{L}_{\text{graph}} = \frac{1}{M} \sum_{j=1}^{N} \sum_{t=1}^{T} \left\| f_{\phi_j}(\mathbf{X} \odot \mathbf{s}_{:,j}) - x_{j,t} \right\|_2 \cdot o_{j,t} + \lambda \left\| \sigma(\mathbf{\Theta}) \right\|_1 \tag{3}$$

where $M = \sum_{j=1}^{N} \sum_{t=1}^{T} o_{j,t}$. By calculating the gradients of $\mathbb{E}_{\mathbf{S}}\left[\mathcal{L}_{\text{graph}}\right]$ over $\theta_{ij}$, we get

$$\frac{\partial}{\partial \theta_{kj}} \mathbb{E}_{\mathbf{S}}\left[\mathcal{L}_{\text{graph}}\right] = \frac{1}{M} \frac{\partial}{\partial \theta_{kj}} \sum_{t=1}^{T} \mathbb{E}_{\mathbf{S}} \sum_{j=1}^{N} \left\| f_{\phi_j}(\mathbf{X} \odot \mathbf{s}_{:,j}) - x_{j,t} \right\|_2 \cdot o_{j,t} + \lambda \left\| \sigma(\mathbf{\Theta}) \right\|_1 \tag{4}$$

$$= \frac{1}{M} \sum_{t=1}^{T} \mathbb{E}_{\{s_{ij}\}_{i \notin \mathcal{G}_k}} \frac{\partial}{\partial \theta_{kj}} \mathbb{E}_{\{s_{ij}\}_{i \in \mathcal{G}_k}} \left\| f_{\phi_j}(\mathbf{X} \odot \mathbf{s}_{:,j}) - x_{j,t} \right\|_2 \cdot o_{j,t} + \lambda \sigma'(\theta_{kj}) \tag{5}$$

$$= \frac{1}{M} \sum_{t=1}^{T} \mathbb{E}_{\{s_{ij}\}_{i \notin \mathcal{G}_k}} \frac{\partial}{\partial \theta_{kj}} \Big( \sigma(\theta_{kj}) \left\| f_{\phi_j}(\mathbf{X} \odot \mathbf{s}_{:,j|\mathcal{G}_k=1}) - x_{j,t} \right\|_2 \cdot o_{j,t} \tag{6}$$

$$+ \left(1 - \sigma(\theta_{kj})\right) \left\| f_{\phi_j}(\mathbf{X} \odot \mathbf{s}_{:,j|\mathcal{G}_k=0}) - x_{j,t} \right\|_2 \cdot o_{j,t} \Big) + \lambda \sigma'(\theta_{kj}) \tag{7}$$

$$= \frac{1}{M} \sum_{t=1}^{T} \mathbb{E}_{\{s_{ij}\}_{i \notin \mathcal{G}_k}} \sigma'(\theta_{kj}) \Big( \lambda + \| e_{NN,i} + e_{t,j} \|_2 \cdot o_{j,t} \tag{8}$$

$$- \left\| f_{\phi_j}(\mathbf{X} \odot \mathbf{s}_{:,j|\mathcal{G}_k=0}) - x_{j,t} \right\|_2 \cdot o_{j,t} \Big) \tag{9}$$

$$\approx \frac{1}{M} \sum_{t=1}^{T} \mathbb{E}_{\{s_{ij}\}_{i \notin \mathcal{G}_k}} \sigma'(\theta_{kj}) \Big( \lambda + e_{t,j}^2 \cdot o_{j,t} - \left(\Delta_{\mathcal{G}_k,j} + e_{t,j}\right)^2 \cdot o_{j,t} \Big) \tag{10}$$

$$= \frac{1}{M} \sum_{t=1}^{T} \mathbb{E}_{\{s_{ij}\}_{i \notin \mathcal{G}_k}} \sigma'(\theta_{kj}) \left( \lambda - \left( 2\Delta_{\mathcal{G}_k,j} e_{t,j} + \Delta_{\mathcal{G}_k,j}^2 \right) \cdot o_{j,t} \right) \tag{11}$$

where $f_{\phi_j}(\cdot)$ is the MPGNN prediction module, $\mathbf{s}_{:,j|\mathcal{G}_k=r}$ is generated with (2), only with $s_{kj} = r$. And we define $\Delta_{\mathcal{G}_k,j}$ as the causal effects of group $\mathcal{G}_k$, i.e.,

$$\Delta_{\mathcal{G}_k,j} = f_{\phi_j}(\mathbf{X} \odot \mathbf{s}_{:,j|\mathcal{G}_k=1}) - f_{\phi_j}(\mathbf{X} \odot \mathbf{s}_{:,j|\mathcal{G}_k=0}) \tag{12}$$

We achieve (4) by changing the order of summation, (5) by eliminating irrelevant terms in CDNN and splitting the summation of $s_{ij}$ where $i$ is in or not in group $\mathcal{G}_k$, (6, 7) by calculating the expectation of Bernoulli distribution, (9) by ignoring $e_{NN,j}$. When we treat observation mask $o_{j,t}$ and noise $e_{j,t}$ as random variables, we get the expectation of the derivatives

$$\mathbb{E}_{o_{j,t}} \mathbb{E}_{e_{j,t}} \frac{\partial}{\partial \theta_{kj}} \mathbb{E}_{\mathbf{S}}\left[\mathcal{L}_{\text{graph}}\right] = \frac{1}{M} \sum_{t=1}^{T} \mathbb{E}_{\{s_{ij}\}_{i \notin \mathcal{G}_k}} \mathbb{E}_{o_{j,t}} \mathbb{E}_{e_{j,t}} \sigma'(\theta_{kj}) \left( \lambda - \left( 2\Delta_{\mathcal{G}_k,j} e_{t,j} + \Delta_{\mathcal{G}_k,j}^2 \right) \cdot o_{j,t} \right) \tag{13}$$

$$= \frac{1}{M} \sum_{t=1}^{T} \mathbb{E}_{\{s_{ij}\}_{i \notin \mathcal{G}_k}} \sigma'(\theta_{kj}) \left( \lambda - \Delta_{\mathcal{G}_k,j}^2 \cdot p \right) \tag{14}$$

Where $p$ is the missing probability. $\sigma'(\cdot)$ is the derivative of the sigmoid function and is always positive.

If group $\mathcal{G}_k$ does not Granger cause $j$, then $|\Delta_{\mathcal{G}_k,j}| \leq \lambda_0$ (Assumption 3). Then setting $\lambda = p\lambda_0^2$ would make (14) expected to be positive, and $\theta_{kj}$ decreases towards $-\infty$, $q_{kj} = \sigma(\theta_{kj})$

decreases towards 0. Similarly, If group $\mathcal{G}_k$ Granger cause $j$, (14) is expected to be negative and $q_{kj} = \sigma(\theta_{kj})$ increases towards 1.

# B Additional Experiments

## B.1 Graph Density

VAR datasets are generated with various graph densities, i.e., $\rho = \sum_{i=1}^{N}\sum_{j=1}^{N} a_{ij}/N^2$ where $\mathbf{A}$ is the adjacency matrix of the causal graph. To further demonstrate our performance in different settings, we perform comparison experiments on VAR with various graph densities, shown in Table 4. We can observe that, the performances of all approaches degrade significantly when graph density increases. However, our CUTS+ still beats all baselines on all graph densities.

Table 1: Performance comparison of CUTS+ on VAR ($N = 128$) with various graph densities $\rho = 0.01, 0.03, 0.05, 0.07, 0.1$. The missingness is set as RM with $p = 0.3$.

| Method | Imput. | **VAR with RM** ($p = 0.3$) | | | | |
|---|---|---|---|---|---|---|
| | | $\rho = 0.01$ | $\rho = 0.03$ | $\rho = 0.05$ | $\rho = 0.07$ | $\rho = 0.1$ |
| NGC | ZOH | 1.0000 ± 0.0000 | 0.8268 ± 0.0103 | 0.6492 ± 0.0112 | 0.5769 ± 0.0104 | 0.5443 ± 0.0089 |
| NGC | TimesNet | 0.9819 ± 0.0046 | 0.7947 ± 0.0165 | 0.6115 ± 0.0084 | 0.5303 ± 0.0066 | 0.5133 ± 0.0058 |
| eSRU | ZOH | 0.9127 ± 0.0118 | 0.7007 ± 0.0114 | 0.5958 ± 0.0041 | 0.5530 ± 0.0074 | 0.5324 ± 0.0043 |
| eSRU | TimesNet | 0.8052 ± 0.0193 | 0.6118 ± 0.0143 | 0.5359 ± 0.0095 | 0.5127 ± 0.0066 | 0.5093 ± 0.0050 |
| SCGL | ZOH | 1.0000 ± 0.0000 | 0.6628 ± 0.0031 | 0.5753 ± 0.0085 | 0.5707 ± 0.0077 | 0.5438 ± 0.0076 |
| SCGL | TimesNet | 1.0000 ± 0.0000 | 0.6510 ± 0.0113 | 0.5792 ± 0.0065 | 0.5642 ± 0.0098 | 0.5394 ± 0.0032 |
| NGM | | 0.7425 ± 0.1035 | 0.5625 ± 0.0339 | 0.5327 ± 0.0156 | 0.5335 ± 0.0121 | 0.5223 ± 0.0078 |
| CUTS | | 0.9998 ± 0.0001 | 0.9376 ± 0.0086 | 0.7470 ± 0.0185 | 0.5655 ± 0.0145 | 0.5315 ± 0.0117 |
| CUTS w C2FD | | 1.0000 ± 0.0000 | 0.9638 ± 0.0069 | 0.7712 ± 0.0195 | 0.5753 ± 0.0073 | 0.5363 ± 0.0068 |
| **CUTS+** | | **1.0000** ± 0.0000 | **0.9907** ± 0.0008 | **0.8630** ± 0.0111 | **0.6460** ± 0.0103 | **0.5844** ± 0.0098 |

## B.2 Scalability

In the main text, we show the scalability of our CUTS+ on VAR and Lorenz-96 datasets. We show more experiments here on VAR and Lorenz-96 with $N = 16, 32, 64, 128, 256, 512$ on 4 different data missing scenarios and without data missing. The results are in Table 3. We observe good scalability with or without data missing when $N$ increases and the performance only degrades clearly when $N = 512$ or $p = 0.6$.

## B.3 Quantitative Comparison on AQI Dataset

Although we do not have access to the ground-truth causal graph because of the extremely complex atmosphere physics in AQI dataset, the geometrical distances are very closely related to the real causal relationships. To show the quantitative result, we take the distance matrix as the ground truth graph, which is calculated as

$$d_{ij} \propto 1/\mathrm{dist}(i, j) \tag{15}$$

After selecting a threshold to binarize the ground truth graph, we perform experiments on AQI dataset with RM ($p = 0.3$). We observe that our causal discovery results are the closest to

Table 2: Performance comparison of CUTS+ on VAR datasets with $N = 16, 32, 64, 128, 256, 512$. The data missing is set as RM with $p = 0, 0.3, 0.6$.

| $N$ | **VAR with RM** | | **VAR with RBM** | | **VAR** |
|---|---|---|---|---|---|
| | $p = 0.3$ | $p = 0.6$ | $p_{\text{blk}} = 0.15\%$ | $p_{\text{blk}} = 0.3\%$ | No missing |
| 16 | 0.9917 $\pm$ 0.0034 | 0.9639 $\pm$ 0.0146 | 0.9931 $\pm$ 0.0038 | 0.9887 $\pm$ 0.0064 | 0.9957 $\pm$ 0.0016 |
| 32 | 0.9916 $\pm$ 0.0028 | 0.9572 $\pm$ 0.0041 | 0.9942 $\pm$ 0.0016 | 0.9923 $\pm$ 0.0023 | 0.9977 $\pm$ 0.0012 |
| 64 | 0.9911 $\pm$ 0.0023 | 0.9577 $\pm$ 0.0094 | 0.9945 $\pm$ 0.0018 | 0.9931 $\pm$ 0.0020 | 0.9972 $\pm$ 0.0014 |
| 128 | 0.9907 $\pm$ 0.0008 | 0.9569 $\pm$ 0.0051 | 0.9939 $\pm$ 0.0018 | 0.9912 $\pm$ 0.0025 | 0.9971 $\pm$ 0.0005 |
| 256 | 0.9893 $\pm$ 0.0031 | 0.9557 $\pm$ 0.0035 | 0.9928 $\pm$ 0.0010 | 0.9903 $\pm$ 0.0018 | 0.9960 $\pm$ 0.0014 |
| 512 | 0.9329 $\pm$ 0.0043 | 0.8496 $\pm$ 0.0043 | 0.9485 $\pm$ 0.0034 | 0.9403 $\pm$ 0.0028 | 0.9647 $\pm$ 0.0039 |

Table 3: Performance comparison of CUTS+ on Lorenz-96 datasets with $N = 16, 32, 64, 128, 256, 512$. The data missing is set as RM with $p = 0, 0.3, 0.6$.

| $N$ | **Lorenz-96 with RM** | | **Lorenz-96 with RBM** | | **Lorenz-96** |
|---|---|---|---|---|---|
| | $p = 0.3$ | $p = 0.6$ | $p_{\text{blk}} = 0.15\%$ | $p_{\text{blk}} = 0.3\%$ | No missing |
| 16 | 0.9999 $\pm$ 0.0001 | 0.9975 $\pm$ 0.0012 | 1.0000 $\pm$ 0.0000 | 0.9999 $\pm$ 0.0002 | 1.0000 $\pm$ 0.0000 |
| 32 | 0.9998 $\pm$ 0.0001 | 0.9962 $\pm$ 0.0023 | 1.0000 $\pm$ 0.0000 | 0.9999 $\pm$ 0.0000 | 1.0000 $\pm$ 0.0000 |
| 64 | 0.9998 $\pm$ 0.0002 | 0.9915 $\pm$ 0.0033 | 0.9997 $\pm$ 0.0002 | 0.9997 $\pm$ 0.0003 | 1.0000 $\pm$ 0.0000 |
| 128 | 0.9992 $\pm$ 0.0002 | 0.9950 $\pm$ 0.0011 | 0.9994 $\pm$ 0.0002 | 0.9992 $\pm$ 0.0002 | 0.9998 $\pm$ 0.0001 |
| 256 | 0.9984 $\pm$ 0.0002 | 0.9911 $\pm$ 0.0017 | 0.9989 $\pm$ 0.0002 | 0.9986 $\pm$ 0.0002 | 0.9997 $\pm$ 0.0000 |
| 512 | 0.9969 $\pm$ 0.0005 | 0.9838 $\pm$ 0.0007 | 0.9975 $\pm$ 0.0002 | 0.9964 $\pm$ 0.0006 | 0.9990 $\pm$ 0.0002 |

the distance matrix, demonstrating the superior performance of CUTS+. The ablation study by comparing CUTS+ with CUTS and "CUTS w C2FD" shows that both C2FD and MPGNN contribute to the performance gain.

However, we would like to clarify that this quantitative experiment may not fully reflect the true causal discovery performance since the distance matrix may not be the actual causal graph.

# C Implementation Details

## C.1 Computation

We conduct experiments on a PC with Intel Core CPUs and NVIDIA GeForce RTX 3090 GPUs. For baseline algorithms such as PCMCI and LCCM, the computation time is extremely long when $N \geq 128$ (more than 12 hrs each task), so we only perform comparisons with PCMCI and LCCM on NetSim and Dream-3 datasets.

## C.2 Datasets

The VAR and Lorenz-96 datasets support setting $N$. To ensure the numbers of causal parents for each time-series in VAR are roughly the same when $N$ changes, the sparsity of the causal matrix is set as $0.2, 0.1, 0.05, 0.03, 0.015, 0.008$ for $N = 16 \sim 512$, respectively.

The 4 data missing scenarios used in the experiments are RM ($p = 0.3/0.6$) and RBM ($p_{\text{blk}} = 0.15\%/0.3\%$). We list the detailed parameter settings in Table 5.

Air Quality (AQI) is a dataset of several air quality features (such as PM2.5, SO2, NO2) from

Table 4: Performance comparison of CUTS+ on VAR ($N = 128$) with various graph densities $d = 0.01, 0.03, 0.05, 0.07, 0.1$. The missingness is set as RM with $p = 0.3$.

| **Met.** | **Imput.** | **AQI with RM** ($N = 128$) $p = 0.3$ | **AQI with RM** ($N = 128$) $p = 0.6$ | **AQI with RBM** ($N = 128$) $p_{\text{blk}} = 0.15\%$ | **AQI with RBM** ($N = 128$) $p_{\text{blk}} = 0.3\%$ | **AQI** ($N = 128$) No missing |
|---|---|---|---|---|---|---|
| NGC | ZOH | 0.xxxx ± 0.xxxx | 0.xxxx ± 0.xxxx | 0.xxxx ± 0.xxxx | 0.xxxx ± 0.xxxx | 0.xxxx ± 0.xxxx |
| | TimesNet | 0.xxxx ± 0.xxxx | 0.xxxx ± 0.xxxx | 0.xxxx ± 0.xxxx | 0.xxxx ± 0.xxxx | |
| eSRU | ZOH | 0.xxxx ± 0.xxxx | 0.xxxx ± 0.xxxx | 0.xxxx ± 0.xxxx | 0.xxxx ± 0.xxxx | 0.xxxx ± 0.xxxx |
| | TimesNet | 0.xxxx ± 0.xxxx | 0.xxxx ± 0.xxxx | 0.xxxx ± 0.xxxx | 0.xxxx ± 0.xxxx | |
| SCGL | ZOH | 0.xxxx ± 0.xxxx | 0.xxxx ± 0.xxxx | 0.xxxx ± 0.xxxx | 0.xxxx ± 0.xxxx | 0.xxxx ± 0.xxxx |
| | TimesNet | 0.xxxx ± 0.xxxx | 0.xxxx ± 0.xxxx | 0.xxxx ± 0.xxxx | 0.xxxx ± 0.xxxx | |
| NGM | | 0.xxxx ± 0.xxxx | 0.xxxx ± 0.xxxx | 0.xxxx ± 0.xxxx | 0.xxxx ± 0.xxxx | 0.xxxx ± 0.xxxx |
| CUTS | | 0.xxxx ± 0.xxxx | 0.xxxx ± 0.xxxx | 0.xxxx ± 0.xxxx | 0.xxxx ± 0.xxxx | 0.xxxx ± 0.xxxx |
| CUTS w C2FD | | 0.xxxx ± 0.xxxx | 0.xxxx ± 0.xxxx | 0.xxxx ± 0.xxxx | 0.xxxx ± 0.xxxx | 0.xxxx ± 0.xxxx |
| **CUTS+** | | **0.xxxx ± 0.xxxx** | **0.xxxx ± 0.xxxx** | **0.xxxx ± 0.xxxx** | **0.xxxx ± 0.xxxx** | **0.xxxx ± 0.xxxx** |

Table 5: Parameter settings for our 4 types of data missing.

| **Setting** | $p$ | $p_{\text{blk}}$ | $L_{\min}$ | $L_{\max}$ |
|---|---|---|---|---|
| No missing | 0 | 0 | / | / |
| RM $p = 0.3$ | 0.3 | 0 | / | / |
| RM $p = 0.6$ | 0.6 | 0 | / | / |
| RBM $P_{\text{blk}} = 0.15\%$ | 0.1 | 0.0015 | 12 | 48 |
| RBM $P_{\text{blk}} = 0.3\%$ | 0.1 | 0.003 | 12 | 48 |

437 monitoring stations spread across 43 Chinese cities[1], with an hourly measurement over one year. We consider PM2.5 pollution index in the dataset, which has minimal missing values among all the features. Those 437 stations can be divided into two parts, respectively distributed in City Cluster A centered around Beijing, and City Cluster B centered around Shenzhen. Here we only use the Cluster B part centered around Shenzhen, which has a lower variance. The total length of the dataset is L = 8760 and the number of nodes is N = 163.

## C.3 Details for Our Approach

We show the key parameters of CUTS+ in Table 6 and discuss some details for implementation in the following.

**Sliding Window Imputation.** For every batch during training, we extract data from a defined temporal window. Then, predictions are performed at each temporal point by utilizing data from historical data. The predicted values gradually replace the missing entries in the original time-series data through the use of the following equation:

$$\tilde{x}_{t,i}^{(m+1)} = \begin{cases} (1-\alpha)\tilde{x}_{t,i}^{(m)} + \alpha\hat{x}_{t,i}^{(m)} & o_{t,i} = 0 \text{ and } m \geq n_1 \\ \tilde{x}_{t,i}^{0} & o_{t,i} = 1 \text{ or } m < n_1 \end{cases} \tag{16}$$

Here $m$ indexes the iteration steps and the update begin after $n_1$ epochs. $\tilde{x}_{t,i}^{(0)}$ denotes the initial data (unobserved entries filled with zero order holder). $\alpha$ is selected to prevent the abrupt change

[1]https://www.microsoft.com/en-us/research/project/urban-computing/

of imputed data. For the missing points, their predicted value $\hat{x}_{t,i}^{(m)}$ is unsupervised with $\mathcal{L}$ but updated to $\tilde{x}_{t,i}^{(m)}$ to obtain a "delayed" error in causal graph inference [3].

**Parameter Tuning.** The hyper-parameters are tuned with grid search on the validation dataset (independently generated with different random seeds and the same size). We did the same for baseline algorithms to maintain fairness.

**Experiments for Time Costs.** To test the time costs for cMLP / cLSTM and CUTS+, we separately implement a simulated optimization process with only ***Prediction Stage***. This CPG and input time-series are randomly generated with Bernoulli and normal distribution. We set the hyperparameters (e.g., layer numbers, size of the hidden layer) as the best-performing combination on VAR datasets. The batch size is set to 128 for three models.

## C.4 Baseline Methods

This work incorporates a lot of baseline methods. We briefly describe the implementation details for reproducibility in the following and show key parameters in Table 7.

**PCMCI.** The code is from `https://github.com/jakobrunge/tigramite`. We use ParCorr as conditional independence tests for all experiments. Although nonlinear tests, e.g., CMIKnn, and GPDC are available, but the computational cost is unacceptable for our high-dimensional settings.

**NGC.** The code is from `https://github.com/iancovert/Neural-GC`. We use the cMLP network because according to the original paper [4] cMLP achieves better performance, except for DREAM-3 dataset.

**eSRU.** The code is from `https://github.com/sakhanna/SRU_for_GCI`.

**SCGL.** The code is downloaded from link shared in its original paper [5].

**LCCM.** The code is from `https://github.com/edebrouwer/latentCCM`.

**NGM.** The code is from `https://github.com/alexisbellot/Graphical-modelling-continuous-time`.

**CUTS.** The code is from `https://github.com/jarrycyx/UNN`. In the ablation study, we add C2FD to CUTS, named "CUTS w C2FD".

**TimesNet.** The code is from `https://github.com/thuml/TimesNet`.

Table 6: Hyperparameters settings of CUTS+ in the aforementioned experiments.

| **Hyperparam.** | **VAR** | **Lorenz** | **DREAM-3** | **AQI** |
|---|---|---|---|---|
| Batch size | 128 | 128 | 128 | 128 |
| Window size | 10 | 1 | 5 | 24 |
| Initial groups | 16 | 32 | 25 | 20 |
| Weight decay | 0.003 | 0 | 0 | 0 |
| GRU layers | 1 | 1 | 1 | 1 |
| Hidden size | 32 | 32 | 32 | 32 |
| Stage 1 Lr | $10^{-3} \to 10^{-4}$ | $10^{-3} \to 10^{-4}$ | $10^{-3} \to 10^{-4}$ | $10^{-3} \to 10^{-4}$ |
| Stage 2 Lr | $10^{-2} \to 10^{-3}$ | $10^{-2} \to 10^{-3}$ | $10^{-2} \to 10^{-3}$ | $10^{-2} \to 10^{-3}$ |
| Gumbel $\tau$ | $1 \to 0.1$ | $1 \to 0.1$ | $1 \to 0.1$ | $1 \to 0.1$ |
| $\lambda$ | $0.01 \to 0.01$ | $0.01 \to 0.01$ | $0.01 \to 0.01$ | $0.01 \to 0.01$ |

Table 7: Hyperparameters settings of the baseline causal discovery and data imputation algorithms.

| Methods | Params. | VAR | Lorenz | NetSim | DREAM-3 |
|---|---|---|---|---|---|
| PCMCI | $\tau_{max}$ | 3 | 3 | 5 | 5 |
| | $PC_\alpha$ | 0.05 | 0.05 | 0.05 | 0.05 |
| NGC | Learning rate | 0.05 | 0.05 | 0.05 | 0.05 |
| | $\lambda_{ridge}$ | 0.01 | 0.01 | 0.01 | 0.01 |
| | $\lambda$ | $0.02 \to 0.2$ | $0.02 \to 0.2$ | $0.04 \to 0.4$ | $0.02 \to 0.01$ |
| eSRU | $\mu_1$ | 0.1 | 0.1 | 0.1 | 0.7 |
| | Learning rate | 0.01 | 0.01 | 0.001 | 0.001 |
| | Batch size | 250 | 250 | 100 | 100 |
| | Epochs | 2000 | 2000 | 2000 | 2000 |
| SCGL | Epochs | 50 | 50 | 50 | 50 |
| | Batch size | 32 | 32 | 32 | 32 |
| | Window | 3 | 3 | 3 | 3 |
| LCCM | Epochs | 50 | 50 | 50 | 50 |
| | Batch size | 10 | 10 | 10 | 10 |
| | Hidden size | 20 | 20 | 20 | 20 |
| NGM | Steps | 2000 | 2000 | 2000 | 2000 |
| | Horizon | 5 | 5 | 5 | 5 |
| | GL_reg | 0.05 | 0.05 | 0.05 | 0.05 |
| | Chunk num | 100 | 100 | 100 | 46 |
| CUTS | $n_1$ | 5 | 50 | 200 | 20 |
| | $n_2$ | 15 | 150 | 600 | 30 |
| | $n_3$ | 30 | 300 | 200 | 50 |
| | $\alpha$ | 0.1 | 0.01 | 0.01 | 0.01 |
| | Input step | 3 | 1 | 5 | 5 |
| | Batch size | 128 | 128 | 128 | 128 |
| | Hidden features | 128 | 128 | 128 | 128 |
| | Network layers | 3 | 3 | 3 | 5 |
| | Weight decay | 0.001 | 0 | 0.001 | 0 |
| | Stage 1 Lr | $10^{-4} \to 10^{-5}$ | $10^{-4} \to 10^{-5}$ | $10^{-4} \to 10^{-5}$ | $10^{-4} \to 10^{-5}$ |
| | Stage 2 Lr | $10^{-2} \to 10^{-3}$ | $10^{-2} \to 10^{-3}$ | $10^{-2} \to 10^{-3}$ | $10^{-2} \to 10^{-3}$ |
| | Gumbel $\tau$ | $1 \to 0.1$ | $1 \to 0.1$ | $1 \to 0.1$ | $1 \to 0.1$ |
| | $\lambda$ | 0.1 | 0.1 | 5 | 5 |

# D Broader Impacts

This work takes into account the high-dimensionality problem which is seldomly focused on by previous works. CUTS+ paves the way toward causal discovery in real applications in which the time-series often contain hundreds of variables. The possible application fields include medicine, healthcare, social science, and finance.

# E Limitations

Our approach, CUTS+, is a Granger-causality-based causal discovery algorithm. A main limitation of our CUTS+ is the gap between Granger causality and real causality. Granger causality may fail when there exists latent confounders or sub-sampled causal effects, which are common in real datasets. Moreover, our CUTS+ handle irregular time-series with missing data imputation module and cannot directly use irregular inputs. The performance may be hampered when the sampling frequency of each time-series is different. We focus on RM and RBM in the experiments, which can be categorized into Missing Complete at Random (MCAR), a most common type

of data missing. However, there are more types of missing that are often considered in causal inference literature [6].

# References


[1] K. Hornik, M. Stinchcombe, and H. White, “Multilayer feedforward networks are universal approximators,” *Neural networks*, vol. 2, no. 5, pp. 359–366, 1989.

[2] Y. Cheng, R. Yang, T. Xiao, Z. Li, J. Suo, K. He, and Q. Dai, “CUTS: Neural Causal Discovery from Irregular Time-Series Data,” in *The Eleventh International Conference on Learning Representations*, Feb. 2023.

[3] W. Cao, D. Wang, J. Li, H. Zhou, L. Li, and Y. Li, “BRITS: Bidirectional recurrent imputation for time series,” in *Advances in Neural Information Processing Systems*, vol. 31, Curran Associates, Inc., 2018.

[4] A. Tank, I. Covert, N. Foti, A. Shojaie, and E. B. Fox, “Neural granger causality,” *IEEE Transactions on Pattern Analysis and Machine Intelligence*, vol. 44, no. 8, pp. 4267–4279, 2022.

[5] C. Xu, H. Huang, and S. Yoo, “Scalable Causal Graph Learning through a Deep Neural Network,” in *Proceedings of the 28th ACM International Conference on Information and Knowledge Management*, CIKM ’19, (New York, NY, USA), pp. 1853–1862, Association for Computing Machinery, Nov. 2019.

[6] T. Geffner, J. Antoran, A. Foster, W. Gong, C. Ma, E. Kiciman, A. Sharma, A. Lamb, M. Kukla, N. Pawlowski, M. Allamanis, and C. Zhang, “Deep End-to-end Causal Inference,” June 2022.
